# Supplementary material for: Unsupervised Video Interpolation by Learning Multilayered 2.5D Motion Fields
Source: arXiv:2204.09900 source file (2022-04-21)
Supplement: Supplementary file 2 [file supplementary.tex]

\date{}
\title{Supplemental Material}
\maketitle

\section{Velocity fields and diffeomorphisms}

Here we provide a brief proof for the forward and backward consistencies of the location mapping stated in Section \ref{section:motion_fields}.

\begin{theorem}\label{theorem}
Let $t_0,t_1,t_2$ be any three timestamps, define
$$ [u_1,v_1]^\top = M(u_0,v_0,t_0,t_1) $$
and $$ [u_2,v_2]^\top = M(u_0,v_0,t_0,t_2), $$then
\begin{equation}
    M\big(M(u_0,v_0,t_0,t_1),t_1,t_2\big) = [u_2,v_2]^\top
\end{equation}
\end{theorem}

\begin{proof}
From Equation \ref{integration} we have
\begin{align}
&[u_2,v_2]^\top - [u_1,v_1]^\top \nonumber\\
&= \int_{t_0}^{t_2} V\big( M(u_0,v_0,t_0,t), t\big)dt - \int_{t_0}^{t_1} V\big( M(u_0,v_0,t_0,t), t\big)dt\\
&= \int_{t_1}^{t_2} V\big( M(u_0,v_0,t_0,t), t\big)dt
\end{align}
Also because
\begin{align}
&M\big(M(u_0,v_0,t_0,t_1),t_1,t_2\big)-[u_1,v_1]^\top \nonumber\\
&=\int_{t_1}^{t_2} V\big( M(u_1,v_1,t_1,t),t\big)dt
\end{align}
Therefore it suffices to show 
\begin{align}
    &\int_{t_1}^{t_2} V\big( M(u_0,v_0,t_0,t),t\big)dt \nonumber \\&= \int_{t_1}^{t_2} V\big( M(u_1,v_1,t_1,t),t\big)dt,
\end{align}
which can be derived from the equality of initial conditions
\begin{align}
    M\big(u_1,v_1,t_1,t\big)|_{t=t_1}=[u_1,v_1]^\top= M(u_0,v_0,t_0,t)|_{t=t_1}
\end{align}
\end{proof}

Hence the location mapping is forward consistent
$$M\big(M(u_0,v_0,t_0,t_1),t_1,t_2\big)= [u_2,v_2]^\top$$
and backward consistent
$$M\big(M(u_0,v_0,t_0,t_1),t_1,t_0\big)= [u_0,v_0]^\top.$$

A mapping $M:\mathbb{R}^2\mapsto \mathbb{R}^2$ is said to be diffeomorphic if: \begin{itemize}
    \item $M$ is everywhere differentiable, and
    \item $M^{-1}$ exists and is everywhere differentiable.
\end{itemize}

By integrating a velocity field w.r.t. time variable in Equation \ref{integration}, one can show the resulting location mapping $M(\cdot, t_0,t_1)$ is always diffeomorphic for all $t_0,t_1$, since the inverse location mapping is already given by backward consistency:
\begin{equation}
    M^{-1}(\cdot, t_0,t_1) = M(\cdot, t_1, t_0).
\end{equation}

Diffeomorphisms, however, are incapable of representing occlusions in videos. To exemplify this limitation, we will consider the following case: in the first frame, two points $A$ and $B$ in the background are divided by an occluder $C$. That is, by connecting a line between these two background point $A$ and $B$, the line passes through the occluder. In the next frame, the occluder moves pass point $B$, hence $C$ is no longer on the line segment between $A$ and $B$, but is instead on its extension. Diffeomorphic motion fields can be considered as spatially smooth deformations. Therefore diffeomorphic location mappings are not able to move $C$ past $A$ or $B$, hence the reason why we need to introduce additional video layers.

\section{Minimal number of video layers for occlusion handling}

\begin{figure}
    \centering
    \includegraphics[width=0.45\textwidth]{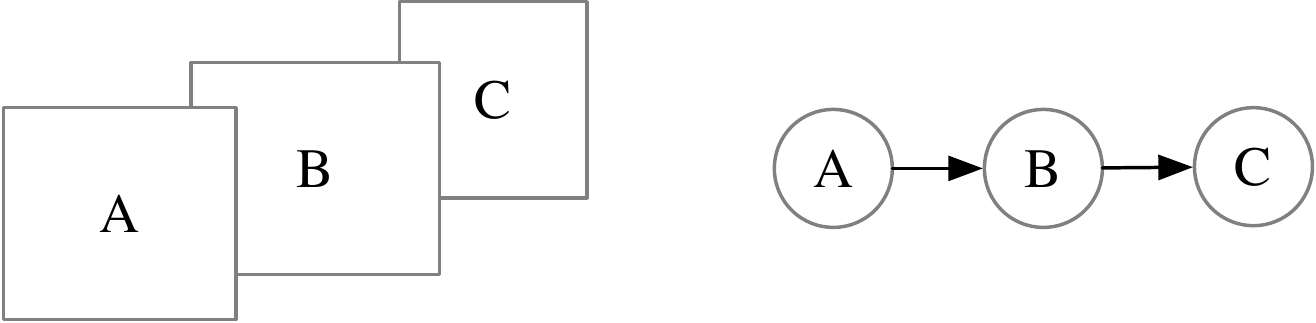}
    \caption{\textbf{DAG representation of occlusions}. On the left shows three objects A, B and C. The order of occlusion can be defined by the graph on the right.}
    \label{fig:occlusion1}
\end{figure}

One convenient way to model occlusions in a scene is by 
a directed acclic graph (DAG). Figure \ref{fig:occlusion1} illustrates an example where the mutual occlusion between three objects is represented by a DAG. 

The minimal number of layers required to model all occlusions in a video corresponds to the maximal length of paths in the DAG. We note, however, for most video clips this number is small. For instance, the example in Figure \ref{fig:occlusion1} can be alternatively represented with a maximum path length of 2, by splitting object B into two halves B1 and B2 as shown in Figure \ref{fig:occlusion12}. This way, one can put A and B2 in the front layer and B1 and C in the back layer and still get away with a two-layer representation.

\begin{figure}
    \centering
    \includegraphics[width=0.45\textwidth]{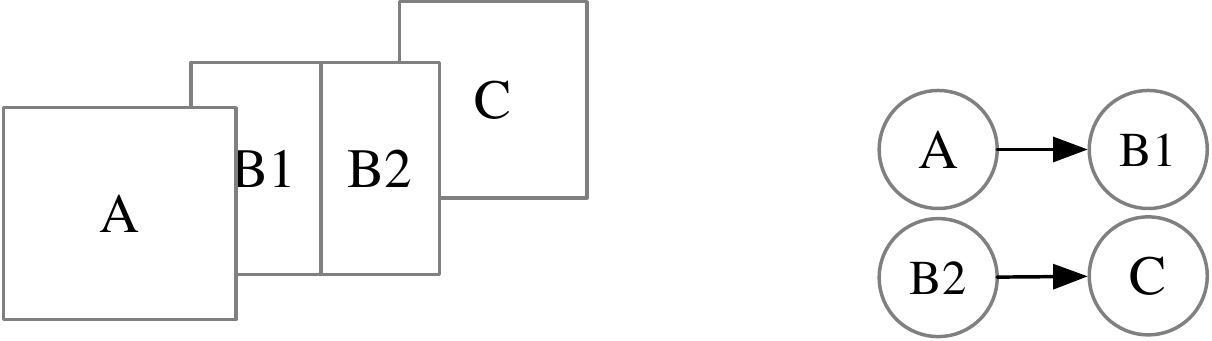}
    \caption{\textbf{An alternative DAG representation}. On the left shows three objects A, B and C. B can be split into two halves B1 and B2, so the corresponding DAG has a maximal path length of 2.}
    \label{fig:occlusion12}
\end{figure}

One limitation of DAG representation, or our layer-wise video representation, is
 that they cannot model any temporal change in the order of occlusions. For example, when A occludes B in the first frame but B occludes A in the second frame. This is because the pseudo-depth of any given pixel is a function of canonical spatial coordinates $u_F,v_F$ and therefore cannot change temporally. One way to overcome this limitation is by representing pseudo-depth as a dynamic function of both spatial coordinates and frame timestamps $t$. We leave this exploration for future work.
